# Supplementary material for: Dynamic Data Layout Optimization with Worst-case Guarantees
Source: arXiv:2405.04984 source file (2024-05-08)
Supplement: Supplementary file 1 [file appendix.tex]

\subsection{Illustration of Reorganization Opportunities}
\label{sec:synexample}
We illustrate the potential performance benefits from dynamic reorganization analytically via a synthetic example. Specifically, we compare the query cost of a static data layout optimized for the entire query sequence to the cost of dynamically switching layouts based on workload changes.

Consider a dataset consisting of $k$ numeric columns $c_1, \ldots, c_k$, where each column contains values that are independently sampled from the uniform distribution $\mathcal{U}(0, 1)$. 
%Note that the data items (i.e. the rows) are uniform random points in $[0,1]^k$. 
The query set consists of point queries with predicates like $p_i$ = $x$, $i\in \{1,...,k\}$ where $x$ is drawn from the distribution $\mathcal{U}(0, 1)$, i.e. asking for data points $p$ whose $i^{th}$ coordinate is $x$. The workload consists of $k$ rounds, %of queries, 
where round $i$ generates $Q$ queries on column %$c_{\pi(i)}$ for $Q$ queries, for some uniformly random permutation $\pi:\, \{1,\ldots, k\} \rightarrow \{1,\ldots, k\}$. 
$c_i$. Suppose that the underlying data storage is an axis-aligned space partitioning structure such as the k-d tree~\cite{bentley1975multidimensional}. In this case, the $[0,1]^k$ data space is partitioned into a set of $k$-dimensional hyper-rectangles $\cB$, whose volume sums to 1. Note that since each column is independently sampled, partitioning based on one column does not improve data skipping on other columns. 

First, consider the static strategy which uses the same set of partitions $\cB$ for all queries. We show that for this query workload, a single data layout does not allow good skipping performance especially for high-dimensional data. Consider a single partition $B \in \cB$ with side lengths $l_1^{(B)}, l_2^{(B)}, \ldots, l_k^{(B)}$. The probability that a query of the form $p_i = x$ hits partition $B$ is exactly the side length $l_i^{(B)}$ in dimension $i$. By linearity of expectation,  the expected number of queries hitting this partition is proportional to $Q \sum_i l_i^{(B)}$.  Each time the partition is hit, a cost proportional to $\mathrm{Vol}(B)$ is incurred since all of the partition's data needs to be read. The expected cost is at least 
\begin{align*}
\sum_{B\in \cB} Q\mathrm{Vol}(B) \sum_{i=1}^k l_i^{(B)} 
&\geq \sum_{B\in \cB} Qk\cdot\mathrm{Vol}(B)^{1+1/k} \geq Qk/ |\cB|^{1/k}.
\end{align*}
The first inequality follows from the Arithmetic Mean-Geometric Mean inequality and the fact that $\mathrm{Vol}(B) = \prod_{i=1}^k l_i^{(B)}$; the second inequality follows from Jensen's inequality and the fact that the total volume of the partitions is equal to 1. 
 Note that the cost without any data skipping is $Qk$. As the dimensionality $k$ gets large, $|\cB|^{1/k}$ tends towards 1, resulting in \emph{almost no savings} from the partitioning. 

In comparison, consider the dynamic strategy of partitioning the entire column $i$ in round $i$ (when column $i$ is queried). This means that column $i$ is divided into $|\cB|$ equal sized intervals, with each interval corresponding to a partition in $\cB$. Now each query in round $i$ only reads one partition in $\cB$ (which has volume $1/|\cB|$), resulting in a total expected cost of $Qk/|\cB|$ over the $k$ rounds of $Q$ queries. The dynamic strategy reduces the query costs by a factor of  $|\cB|^{1-1/k}$ compared to the static one, which is roughly $|\cB|$ as $k$ gets large.

% One key ingredient we did not discuss in this example is the cost of reorganization. In practice, the difficulty lies in deciding whether the performance benefits of a new layout are worth the reorganization cost. 
% In the next section, we discuss how prior works have tackled this problem using online learning algorithms.

\subsection{Preliminary Multi-Table Results}
\label{app:DIP}
In this section, we present our preliminary experiments on using \sysname in a multi-table setup.  

\subsubsection{Implementation Details} We implement a simplified multi-table layout generation scheme inspired by MTO~\cite{ding2021instance}. Instead of independently optimizing each table’s layout, multi-table layout schemes leverage additional information about the joins through Data-Induced Predicates (DIPs)~\cite{dipSri2019} to further improve data-skipping performance. 

To illustrate, consider a scenario involving a dimension and a fact table. A query on the dimension table creates a set of local predicates. Using metadata of the partitions satisfying these local predicates, we can generate additional predicates (DIPs) that capture the range of join column values in the partitions. These DIPs can then be propagated to the fact table via the primary-foreign key relationship. This process effectively translates predicates on one table to data-skipping opportunities in its join tables. 

For our experiments, we have limited our implementation to handle DIPs through one level of join. We included an extra query transformation step that augments fact table queries with DIPs generated from dimension tables. The \layout is agnostic to whether a predicate is induced. The \reorg uses the transformed query to evaluate layout savings and make reorganization decisions. Hence, our implementation did not require modifications to \sysname's layout management and reorganization components.

\subsubsection{Performance Evaluation}
%We have described implementation details and compared perforamnce of \sysname on datasets in their denornalized form with one table in section~\ref{subsec:comp_methods}. In this section, we will implement and evaluate \sysname for dataset with multiple tables. 
%

%Unlike in the single-table data setup, which has one \layout and one set of candidate data layouts, 
%The total budget for partitions is divided among the tables proportional to their size. 
We follow a similar setup to that in \S~\ref{sec:eval-setup}. We compare \sysname with both offline (Static) and online (Periodic and Regret) baselines, using the TPC-H dataset at a scale factor of 10 and a skew factor of 2. A total budget of 100 partitions was split across all tables proportional to their sizes, with each partition containing 700,000 to 2 million rows. We use the same TPC-H workload and reorganization cost ($\alpha=80$) as in the main experiments. In the multi-table setup, each table independently runs its own instance of \sysname. \autoref{tab:dip} reports the logical query and movement costs on the largest lineitem table using two layout generation schemes. 

We observe that single-table layout schemes, such as the Qd-tree, offer negligible performance benefits in dynamic reorganization compared to the best static layout. This is because the layout management and reorganization components can only utilize a subset of queries that have predicates on the lineitem table. In comparison, the total query costs for all methods decrease when input queries are augmented with DIPs. \sysname remains competitive and reduces the total query costs by up to 9.4\% compared to the best static layout, which is generated using the entire query workload. These findings are in line with those from our main experiments.

% Since a query can now contain predicates on different tables, the \layout only processes predicates relevant to its table.

%We experiment with two settings. In the first setting, query workload input for a table's layout manager contains only the predicates with fields from that table's columns. As the algorithm progresses, each table re-organizes its partitions within its own set of budget. Because the \textit{lineitem} table had the largest size, thus, taking up the maximum partition budget, it shows the most variability in performance across algorithms. \autoref{tab:dip} summarizes the performance of one of the tables, \textit{lineitem}.

%This first approach to implementation fails to exploit the dependencies between table which are formed due to joins. In the second setting of our experiments, apart from the input predicates described in setting I, DIPs~\cite{dipSri2019} are also added to the input.  This helps maximize skipping on the fact table. Results in \autoref{tab:dip} measure total cost achieved over one fact table \textit{lineitem} corresponding to two dimension tables, namely, \textit{order} and \textit{part}. Contrasting these results with Graph (i) in \autoref{tab:dip}, the total query cost has decreased for \sysname as well as the baselines. The partition skipping gains is expected to increase as the skewness of the data increases. 

\begin{table}[t]
\caption{Comparison of query and movement cost on the \texttt{lineitem} table in the TPC-H dataset. Multi-table layout scheme that leverages DIPs demonstrates more gains from dynamic reorganization. }
\begin{center}
\footnotesize
\begingroup
\setlength{\tabcolsep}{2pt} % Default value: 6pt
 % Default value: 1
\begin{tabular}{l l l l l l l l}
    \toprule
     & \multicolumn{3}{c}{\textbf{Qd-tree}} & & \multicolumn{3}{c}{\textbf{Qd-tree+DIP}} \\
    \cmidrule{2-4} \cmidrule{6-8}
     & Total & Query  &  Reorg  & & Total & Query  & Reorg  \\
     \midrule
        Static & 15324 & 15324 & 0 & & 13037 & 13037 & 0  \\
        \sysname & 15355  & 14715 & 640 & & 11815  & 10855 & 960  \\
        Periodic & 14869  & 14149 & 720 &  & 13031 & 10471 & 2560  \\
        Regret & 14703 & 14303  & 400 & & 11565  & 11085 & 480 \\
    \bottomrule

\end{tabular}
\endgroup
\label{tab:dip}
\end{center}
\end{table}

\subsection{MTS for Two-state Asymmetric Costs}
In this section, we show that a variant of the classic {\sc MTS} algorithm~\cite{BLS92} also works for two-state asymmetric costs. Following~\cite{bruno2007online}, we assume there exists two states, $s_0$ and $s_1$, where the cost of moving $s_0$ to $s_1$ is 1, but the cost of moving $s_1$ to $s_0$ is 0.

\begin{theorem}
The classic {\sc MTS} algorithm~\cite{BLS92} is 6-competitive for two-state MTS with asymmetric costs.
\end{theorem}

\begin{proof}
Let $\cA_{OPT}$ be the optimal algorithm. Consider a single phase of the classic algorithm. If $\cA_{OPT}$ switches states more than once, then it incurs a cost of at least 1, while classic incurs a cost of 1 from each state, and at most 1 from transitioning states. So the competitive ratio is 3. Now consider the case for when $\cA_{OPT}$ switches states at most once, and consider two consecutive phases of the classic algorithm. 

In this case, there are 8 different possibilities, corresponding to the two different state transitions that $\cA_{OPT}$ could perform. For example, $\cA_{OPT}$ can start in $s_1$ and transition to $s_0$ in the first phase, and go from $s_0$ to $s_1$ in the second phase. Across all 8 different possibilities, $\cA_{OPT}$ incurs cost at least 1. In each possibility, classic incurs a cost of at most 6 across the two phases. Thus the competitive ratio of the classic algorithm is 6.
\end{proof}

\revision{\subsection{Extension: Maintaining Multiple Layouts in Parallel}
In this work, we assume that we do not have additional storage budget to maintain multiple layouts on the same datasets, except temporarily during the background reorganization. However, if we can afford to store multiple physical copies of the data simultaneously, each with a distinct layout or state, we can extend \textsc{OReO} in the following way (without considering load balancing implications).

Suppose we are in the state where the set $\cS$ of layouts does not change. One variant of the algorithm would be to keep $q$ randomly chosen states around in parallel, and switch only when \emph{all states} have cost $>\alpha$. To handle queries, we assign them to the state with the lowest accumulated cost or counter thus far. Let $\cS_A$ be the set of states in $\cS$ which do not currently have their counters filled, and let $f(k)$ be the expected cost of our algorithm when $|\cS_A|=k$. We have \[f(k) \leq q * \alpha + \alpha + \sum_{i=0}^{k-q} f(i)*p_{i, k, q}\], where $p_{i, k, q}$ is the probability that the ${i+1}^{st}$ worst state of the $k$ states was chosen in our set of $q$ states. This is because:
\squishitemize
    \item It takes $q\cdot\alpha$ to completely change to a new set of states.
    \item It takes $\alpha$ cost to query before we switch to a new set of states. We only perform queries on the best of the $q$ states at any given time, and we
stop when the best state's counter reaches $\alpha$.
    \item When we do change to a set of new states, we have $q$ "chances" to land at a state that has cheap expected cost. So $p_{i, k, q}= \frac{\binom{k-i-1}{q-1}}{\binom{k}{q}}$.
\squishend

The number of states maintained in parallel, denoted as $q$, presents a tradeoff between query and reorganization costs. If $q = |\cS|$ then we always get the best query cost, but it costs $q\cdot\alpha$ to reorganize each phase.
If $q=1$ then we rarely get the best query cost, but the expected query and reorganization cost is about $2\log(\alpha)$ in expectation. The best tradeoff likely lies between these extremes.

Another variant of the algorithm would be to switch to a new state whenever one of the $q$ different states reach counter cost $\alpha$. These variants presents an interesting opportunity for future work.}
